# Supplementary material for: Neutrino Intensity Interferometry: Measuring Proto-neutron Star Radii During Core-Collapse Supernovae
Source: arXiv:1704.00010 ancillary file (2017-11-01)
Supplement: Supplementary file 1 [file NeutrinoIntensityInterferometryDerivations.pdf]

# Neutrino intensity interferometry: Measuring proto-neutron star radii during core-collapse supernovae *Supplemental Material*

Warren P. Wright* and James P. Kneller†
*Department of Physics, North Carolina State University, Raleigh, North Carolina 27695, USA*
(Dated: May 26, 2017)

## INTRODUCTION

These supplemental notes are intended to give further detail regarding some of the equations given in the paper *Neutrino intensity interferometry: Measuring proto-neutron star radii during core-collapse supernovae.*

## EQUATIONS 2 TO 4

We begin with a standard wave packed description of the wave function from Eq. (1)

$$\psi_{\vec{p}_0}(x) = \int \frac{d^3p}{(2\pi)^{3/2}} \left(2\pi\sigma_p^2\right)^{-\frac{3}{4}} e^{-\frac{(\vec{p}-\vec{p}_0)^2}{4\sigma_p^2}} e^{-i(E(\vec{p})t-\vec{p}\cdot\vec{x})}. \tag{15}$$

Using $\vec{u} = \vec{p} - \vec{p}_0$ the exponent of the integrand becomes

$$-\frac{\vec{u}^2}{4\sigma_p^2} + i\vec{u}\cdot\vec{x} + i\vec{p}_0\cdot\vec{x} - itE(\vec{p}). \tag{16}$$

With an expansion to second order in $\vec{u}$ and with $E = E(\vec{p}_0)$, $E(\vec{p})$ can be written as

$$E(\vec{p}) = \sqrt{\vec{p}^{\,2} + m^2} \approx E + \frac{\vec{p}_0\cdot\vec{u}}{E} + \frac{1}{2}\sum_{i,j=1}^{3} H_{ij}u_iu_j \tag{17}$$

with $H_{ij} = \left(\delta^i_j E^2 - p_{0,i}p_{0,j}\right)/E^3$ being the hessian matrix. Yielding:

$$\psi_{\vec{p}_0}(\vec{x},t) = \frac{e^{-i(Et-\vec{p}_0\cdot\vec{x})}}{\left(2\pi\sigma_p^2\right)^{3/4}(2\pi)^{3/2}} \int d^3u\ \exp\left[-\frac{1}{2}\sum_{i,j=1}^{3} A_{ij}u_iu_j + \sum_{j=1}^{3} K_ju_j\right] \tag{18}$$

with $A_{ij} = \delta^i_j \frac{1}{2\sigma_p^2} + itH_{ij}$ and $K_j = i\left(x_j - t\,p_{0,j}/E\right)$. This Gaussian integral gives:

$$\psi_{\vec{p}_0}(\vec{x},t) = \frac{e^{-i(Et-\vec{p}_0\cdot\vec{x})}}{\left(2\pi\sigma_p^2\right)^{3/4}(2\pi)^{3/2}} \sqrt{\frac{(2\pi)^3}{\det(A)}}\, e^{\frac{1}{2}\vec{K}^T A^{-1}\vec{K}}. \tag{19}$$

Where

$$A^{-1}_{ij} = \frac{E\sigma_p^2\left(\delta^i_j\left(2E^3 + 4i\,t\,m^2\sigma_p^2\right) + 4\,i\,t\,\sigma_p^2\,p_{0,i}\,p_{0,j}\right)}{\left(E + 2i\,t\,\sigma_p^2\right)\left(E^3 + 2i\,t\,m^2\,\sigma_p^2\right)} \tag{20}$$

$$\det(A) = \left(\frac{1}{2\sigma_p^2} + \frac{i\,t}{E}\right)^2 \left(\frac{1}{2\sigma_p^2} + \frac{i\,t\,m^2}{E^3}\right). \tag{21}$$

After simplification, the resulting wave-function (given in Eqs. (2) to (4)) is

$$\psi_{\vec{p}_0}(\vec{x},t) = \frac{(2\pi)^{-\frac{3}{4}}}{\sigma_\perp(t)\sqrt{\sigma_\parallel(t)}} \exp\left[i\left(\vec{p}_0\cdot\vec{x} - E\,t\right) - \frac{\vec{B}^2}{4\sigma_x\sigma_\perp(t)} - \frac{i\,t\left(\vec{B}\cdot\vec{p}_0\right)^2}{8\,E^3\,\sigma_x^2\,\sigma_\perp(t)\ \sigma_\parallel(t)}\right], \tag{22}$$

where

$$\sigma_\perp(t) = \sigma_x + \frac{i\,t\,\sigma_p}{E}\ ,\ \ \sigma_\parallel(t) = \sigma_x + \frac{i\,t\,\sigma_p}{E\,\gamma^2}\ ,\ \ \sigma_x \equiv \frac{1}{2\sigma_p}\ ,\ \ \vec{B} = \vec{x} - \vec{v}t\ ,\ \ \vec{v} = \vec{p}_0/E\ ,\ \text{ and } \gamma = E/m. \tag{23}$$

It is interesting to note that the parallel spreading of the wave packet is suppressed by two powers of $\gamma$ when compared to the perpendicular spreading. One power of $\gamma$ accounts for the Lorentz contraction of the distance traveled ($\sim tc$), the other power is for the Lorentz contraction of the the parallel size of the wave packet. Another way of thinking about it is simply to replace the $\gamma$ by expressions of energy and mass, thereby showing that the parallel spreading is mass dependent which makes intuitive sense when the photon limit is taken (photon wave packets don't get thicker).

## EQUATION 8 AND $C_2 = 1 \pm \cos\theta\,\mathrm{sech}\,2\Delta$

We begin with Eq. (8) and insert Eq. (6) to obtain

$$C_2 = 1 \pm \frac{\psi_{11}^*\psi_{22}^*\psi_{12}\psi_{21} + \psi_{12}^*\psi_{21}^*\psi_{11}\psi_{22}}{|\psi_{11}|^2|\psi_{22}|^2 + |\psi_{12}|^2|\psi_{21}|^2}, \tag{24}$$

$$= 1 \pm \frac{e^{\chi_s^*}e^{\chi_s^*}e^{\chi_l}e^{\chi_l} + e^{\chi_l^*}e^{\chi_l^*}e^{\chi_s}e^{\chi_s}}{|e^{\chi_s}|^2|e^{\chi_s}|^2 + |e^{\chi_l}|^2|e^{\chi_l}|^2}. \tag{25}$$

Using $\chi_s = \mathrm{Re} + i\ \mathrm{Im}_s$ and $\chi_l = \mathrm{Re} + \Delta + i\ \mathrm{Im}_l$ yields

$$C_2 = 1 \pm \frac{1}{2}\left(e^{i2(\mathrm{Im}_l - \mathrm{Im}_s)} + e^{-i2(\mathrm{Im}_l - \mathrm{Im}_s)}\right)\frac{2}{e^{2\Delta} + e^{-2\Delta}} = 1 \pm \cos\theta\,\mathrm{sech}\,2\Delta \tag{26}$$

with $\theta = 2\,(\mathrm{Im}_l - \mathrm{Im}_s) = 2(\mathrm{Im}\,[\chi_l] - \mathrm{Im}\,[\chi_s])$ and $\Delta = \mathrm{Re}\,[\chi_l] - \mathrm{Re}\,[\chi_s]$.

## EQUATION 9

Using the assumptions outlined at the beginning of the section: *Two Dimensional Illustration*, the definition of $\chi_{ij}$ from Eq. (4) and the definition $\theta = \mathrm{Im}\,[\chi]$ where $\chi = \chi_{11} + \chi_{12}^* + \chi_{21}^* + \chi_{22}$, we derive that

$$\theta = \frac{\sqrt{\gamma^2 - 1}\,E}{4\gamma^3\,(\gamma^2 - 1)\ E^2\,\sigma_x^4 + \gamma L^2}\Big[4\,\gamma^2\,E^2\,\sigma_x^4\,(\gamma^2 - 1)\left(\sqrt{(d-2R)^2 + 4L^2} - \sqrt{(d+2R)^2 + 4L^2}\right) \tag{27}$$

$$-L^2\ (\gamma^2 - 1)\left(\sqrt{(d-2R)^2 + 4L^2} - \sqrt{(d+2R)^2 + 4L^2}\right) - 2\gamma^2 dLR\Big]. \tag{28}$$

In the astrophysical limit, one can expand the square root terms as

$$\sqrt{(d-2R)^2 + 4L^2} - \sqrt{(d+2R)^2 + 4L^2} = -\frac{2dR}{L} + \frac{d^3R}{4L^3} + \frac{dR^3}{L^3} + O\left(\frac{1}{L^5}\right). \tag{29}$$

Together with $\gamma^2 - 1 \to \gamma^2$ this yields,

$$\theta \approx \frac{dER\left[4\,\gamma^4\,E^2\,\sigma_x^4\left(d^2 - 8L^2 + 4\,R^2\right) - \gamma^2\,L^2\left(d^2 + 4\,R^2\right) - 8\,L^4\right]}{4\,L^3\,(4\,\gamma^4\,E^2\sigma_x^4 + L^2)}. \tag{30}$$

Lastly, we once again apply the astrophysical limit to set $d^2 - 8L^2 + 4R^2 \to -8L^2$ and $d^2 + 4R^2 \to 4R^2$ which gives

$$\theta \approx -2\frac{dER}{L}\left(1 + \frac{\gamma^2R^2/2}{4\gamma^4E^2\sigma_x^4 + L^2}\right). \tag{31}$$

This is Eq. (9) and is a simplified form which is very accurate for astrophysical neutrinos.

## EQUATION 10

Once again, using the assumptions outlined at the beginning of the section: *Two Dimensional Illustration*, the definition of $\chi_{ij}$ from Eq. (4) and the definition $\Delta = \mathrm{Re}\left[\chi_l\right] - \mathrm{Re}\left[\chi_s\right]$ where $\chi_s = \chi_{11} = \chi_{22}$ and $\chi_l = \chi_{21} = \chi_{12}$, we derive that

$$\Delta = \frac{\gamma^2\left(\gamma^2-1\right)E^2\sigma_x^2\left[L\left(\sqrt{(d-2R)^2+4L^2}-\sqrt{(d+2R)^2+4L^2}\right)+2dR\right])}{4\,\gamma^2\left(\gamma^2-1\right)\,E^2\,\sigma_x^4+L^2}. \tag{32}$$

Upon applying Eq. (29) and $\gamma^2 - 1 \to \gamma^2$ we obtain

$$\Delta \approx -\frac{\gamma^4 dE^2R\sigma_x^2\left(d^2+4R^2\right)}{4L^2\left(4\gamma^4E^2\sigma_x^4+L^2\right)} \tag{33}$$

We apply the astrophysical limit again to set $d^2 + 4R^2 \to 4R^2$ to get the desired form of Eq. (10):

$$\Delta \approx -\frac{d\,R^3}{4\,L^2\,\sigma_x^2}\frac{4\,E^2\,\gamma^4\,\sigma_x^4}{4\,E^2\,\gamma^4\,\sigma_x^4+L^2}. \tag{34}$$

## EQUATION 13

Starting from the definitions for the size of the wave-packet and asserting that $t = L$ gives

$$|\sigma_\||^2 = \sigma_x^2 + \frac{L^2}{4\,E^2\,\sigma_x^2\,\gamma^4} = \sigma_x^2\frac{4\,E^2\,\sigma_x^4\,\gamma^4+L^2}{4\,E^2\,\sigma_x^4\,\gamma^4}$$
$$|\sigma_\perp|^2 = \sigma_x^2 + \frac{L^2}{4\,E^2\,\sigma_x^2} \approx \frac{L^2}{4\,E^2\,\sigma_x^2}$$

where we assume that $L^2 \gg 4E\sigma_x^4$ in the last line. This is true in the astrophysical context and allows us to write

$$|\Delta| \approx \frac{dR^3}{4L^2\,\sigma_\|^2} \tag{35}$$

$$\theta \approx \theta_{\mathrm{HBT}}\left(1+\frac{\sigma_\perp^2}{\gamma^2\,\sigma_\|^2}\frac{R^2}{2\,L^2}\right) \tag{36}$$

where we have omitted the absolute value signs around $\sigma_\perp$ and $\sigma_\|$ for notational convenience. Thus for small $|\Delta|$ and for $\theta \approx \theta_{\mathrm{HBT}}$ we see that Eq. (13) must be true.

## EQUATION 14

After a wave-packet has spread out considerably, the following approximation becomes relevant in describing the 99% ($3\sigma$) longitudinal thickness

$$3|\sigma_\|| \approx \frac{3\,L}{2\,E\,\sigma_x\,\gamma^2} = \frac{3\,L\,m_\nu^2}{2\,\sigma_x\,E^3}. \tag{37}$$

By dividing by the speed of light and upon inserting the necessary constants, the following expression can be obtained

$$\tau_{\mathrm{coh}} \approx 300 \times 30\ \mathrm{ns}\left(\frac{m_\nu}{0.1\ \mathrm{eV}}\right)^2\left(\frac{L}{10\ \mathrm{kpc}}\right)\left(\frac{15\ \mathrm{MeV}}{E_\nu}\right)^3\left(\frac{100\ \mathrm{fm}}{\sigma_x}\right) \tag{38}$$

Given a number of detected events $n$, over a time period $T$, then the probability of observing an event in a particular experimental bin $\tau_{\mathrm{bin}}$ is $P_1 = n\tau_{\mathrm{bin}}/T$. The probability of observing two events in a particular experimental bin is

$P_2 = P_1^2 = n^2\tau_{\rm bin}^2/T^2$. The probability that those two events were HBT-correlated is $\sim \tau_{\rm coh}/\tau_{\rm bin}$. Therefore, the probability of a pair of HBT-correlated events in a particular experimental bin is

$$P_{HBT} = P_2\,\frac{\tau_{\rm coh}}{\tau_{\rm bin}} = \frac{n^2\tau_{\rm bin}^2}{T^2}\,\frac{\tau_{\rm coh}}{\tau_{\rm bin}} \tag{39}$$

$$= \frac{n^2}{T^2}\,\tau_{\rm coh}\tau_{\rm bin}. \tag{40}$$

Multiplied by the number of experimental bins gives the number of pair HBT-correlated events detected as

$$N_{HBT} = P_{HBT}\,\frac{T}{\tau_{\rm bin}} = n^2\,\frac{\tau_{\rm coh}}{T}. \tag{41}$$

By combining this with Eq.(38) and inserting the appropriate constants one arrives at Eq.(14). One point of clarification in the above formalism is that if $\tau_{\rm coh} > \tau_{\rm bin}$, then it is better to redefine the experimental bins such that $\tau_{\rm bin} = \tau_{\rm coh}$ to maximize the detected interference signal (and avoid unrealistic probabilities). Furthermore, there is a third time scale $\tau_{\rm lc}$, which is the light-crossing time of the detector. The above analysis is true for the case when $\tau_{\rm bin}$ is greater than the time the neutrino spends in the detector, $\tau_{\rm lc} + \tau_{\rm coh}$. Should this not be the case, a different approximation to the probability that two events are HBT-correlated would be needed, and the result would then have a dependence on $\tau_{\rm bin}$.

* wpwright@ncsu.edu
† jpknelle@ncsu.edu
